# Supplementary material for: Conductivity spectrum of ultracold atoms in an optical lattice
Source: arXiv:1712.09965 ancillary file (2019-02-12)
Supplement: Supplementary file 1 [file AndersonSM.pdf]

# Supplementary Material for "Conductivity spectrum of ultracold atoms in an optical lattice"

Rhys Anderson,[1] Fudong Wang,[1] Peihang Xu,[1] Vijin Venu,[1]
Stefan Trotzky,[1] Frédéric Chevy,[2] and Joseph H. Thywissen[1,3]

[1]*Department of Physics, University of Toronto, Ontario M5S 1A7 Canada*
[2]*Laboratoire Kastler Brossel, ENS-PSL Research University, CNRS, UPMC-Sorbonne Universités, Collège de France*
[3]*Canadian Institute for Advanced Research, Toronto, Ontario M5G 1M1 Canada*

## CONTENTS

S1. Experimental techniques 1
  A. Sample preparation 1
  B. Force calibration 2
  C. Finite-time broadening 2

S2. Properties of conductivity 3
  A. Calorimetry and Joule's Law observation 3
  B. Tensor response 4

S3. Eigenspectrum for lattice plus parabolic potential 5

S4. f-sum in continuum and single-band Hubbard models 6
  A. Continuum 6
  B. f-sum in the Hubbard model 7
  C. Relation of f-sum to effective mass 8
  D. Effect of the harmonic trap 9

S5. Kinetic model 10
  A. High-frequency limit 10
  B. Collisional damping in a lattice 12
  C. Impulse response 12
  D. Scattering integral 14

  References 16

## S1. EXPERIMENTAL TECHNIQUES

### A. Sample preparation

The sample is prepared starting from a balanced mixture of $|F, m_F\rangle = |9/2, -9/2\rangle$ and $|F, m_F\rangle = |9/2, -7/2\rangle$ potassium ($^{40}$K) atoms, in a mixture with $|F, m_F\rangle = |1, 1\rangle$ rubidium ($^{87}$Rb) atoms, both confined in a crossed optical dipole trap (XDT). The rubidium atoms are preferentially evaporated away by lowering the depth of the trap, leaving $\sim 1.5 \times 10^5$ potassium atoms in each spin state at a typical temperature of $0.1T_F$. Atom number is typically reduced to $1.0 \times 10^4$ by further evaporation, but varied between $5.0 \times 10^3$ and $5.0 \times 10^4$ for the $N$ dataset. The spin mixture is loaded into a three-dimensional optical lattice of variable depth. The lattice beam profiles are Gaussian, with waists of $60\,\mu$m for the horizontally-propagating beams, and $85\,\mu$m for the vertical lattice. The dipole trap beams are highly elliptical, with waists of $45\,\mu$m by $200\,\mu$m. The dipole trap beams therefore provide the dominant confinement (typically 220 Hz) in the vertical ($z$) direction, but the radial ($xy$) harmonic confinement $\omega_0$ is a combination of the $\omega_{\mathrm{XDT}}$ =32(1) Hz provided by the dipole traps and additional confinement from the lattice beams.Lattice loading and most datasets are taken in uniform field of 20 G with scattering length $180\,a_0$ between spin states, except when the scattering length is intentionally tuned in the $a_s$ set using the s-wave Feshbach resonance located at 202.1G.

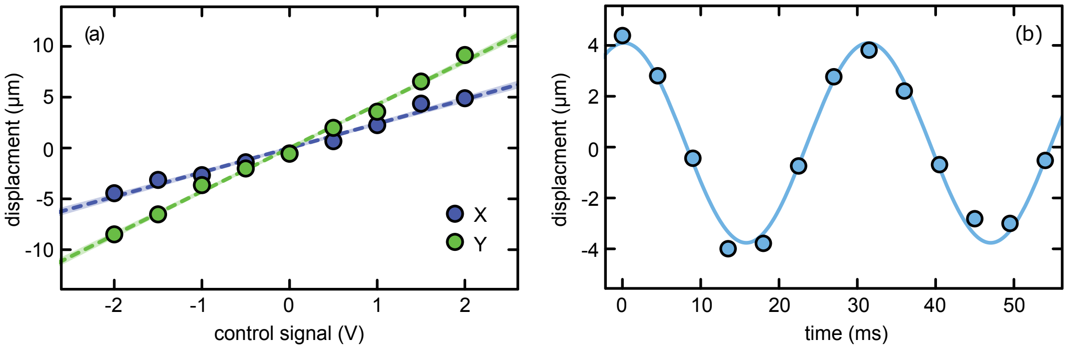


FIG. S1. **Calibration of applied forcing**. (a) The c.m. position of the atomic cloud, with no lattice present, is measured for each control voltage, which is then amplified and sent to piezo-electric mirrors along the beam path of each beam. (b) The spring constant is determined using the known mass of the atom and the free oscillation frequency in the trap.

The imaging process photo-associates atoms in doubly occupied sites [S1, S2]. In order to minimize this effect, we work in a low-filling regime, with typical $\langle n_\uparrow \rangle = \langle n_\downarrow \rangle = 0.12(1)$ per spin state, and average doublon fraction of only 0.02(1). A further reduction of this systematic could use the approach described in [S3, S4].

### B. Force calibration

A force is applied to the sample using displacement $d_\beta(t)$ of the center of the crossed dipole trap (XDT) along direction $\beta$, resulting in a force $F_\beta = m\omega_{\mathrm{XDT}}^2 d_\beta(t)$. Control of the displacement comes from two piezo-electric mirrors reflecting each of the dipole-trap beams into the vacuum chamber. Displacement in $z$ is neither measured nor expected since forces are applied in the $xy$ plane, and no Hall response is anticipated. Typical calibration data is shown in Fig. S1(a), where the center of mass of the atomic cloud is imaged after static displacement of the mirror, by the indicated control signal. The displacement is simply linear in the voltage, with a coefficient determined by the fit. The spring constant $m\omega_{\mathrm{XDT}}^2$ is calibrated with a measurement of the natural oscillation frequency of the cloud, for which typical data is shown in Fig. S1(b). Powers of the beams are chosen for a rotational symmetry of the in-plane oscillation frequencies, with a precision of $\sim 1\,\mathrm{Hz}$.

### C. Finite-time broadening

Force is applied in a time sequence that begins with a $t_1 = 150\,\mathrm{ms}$ linear ramp in amplitude, followed by a period of constant drive force, $t_2 + t_d$ where $t_2 = 50\,\mathrm{ms}$ and $t_d$ is the variable additional drive time of up to two oscillation periods. The finite time of force application sets a lower bound for the spectral width of the response. In order to investigate this effect, we vary the prior modulation time $t_< = t_1 + t_2$ and measure the center-of-mass response of the system in a pure crossed dipole trap. Using a dipole trap with no lattice should decouple the c.m. mode from atom-atom interactions [S5], isolating the Fourier-limited response. Otherwise, we proceed as if measuring conductivity $\sigma(\omega)$: freezing the c.m. motion by snapping on the lattice, isolating four central planes, and measuring the c.m. of the fluorescence distribution.

Widths are determined by fitting the spectra using the expected response function for a damped harmonic oscillator

$$\sigma(\omega) = i\sigma_{\mathrm{amp}} \frac{\Gamma\omega}{\omega^2 - \omega_{\mathrm{XDT}}^2 + i\Gamma\omega} \tag{S1}$$

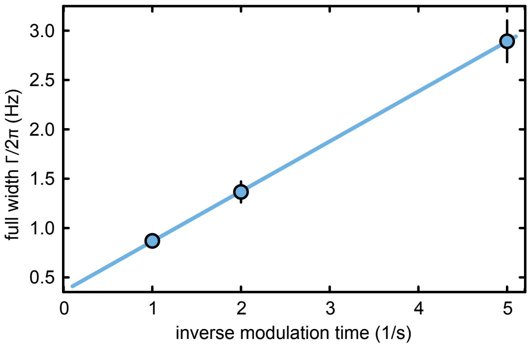


FIG. S2. **Ramp-time-dependent broadening**. The best-fit full width $\Gamma$ is shown versus the inverse modulation time $1/t_<$. Each point corresponds to a spectrum taken with a different time sequence, as described in the text. The solid line is a linear fit to the data, with slope 0.51(1) and offset $2\pi \times 0.36(1)\,\mathrm{Hz}$.

where $\sigma_{\mathrm{amp}}$ is the amplitude, $\omega$ is the drive frequency, $\omega_{\mathrm{XDT}}$ is the trap frequency, and $\Gamma$ is the full width at half

maximum of the c.m. response function. Figure S2 shows the best-fit $\Gamma$ for three spectra, with prior modulation times $t_< = 200\,\mathrm{ms}$ ($150\,\mathrm{ms} + 50\,\mathrm{ms}$), $t_< = 500\,\mathrm{ms}$ ($400\,\mathrm{ms} + 100\,\mathrm{ms}$), and $t_< = 1000\,\mathrm{ms}$ ($900\,\mathrm{ms} + 100\,\mathrm{ms}$). As expected, $\Gamma$ is proportional to the inverse modulation time, $1/t_<$. The data also have a finite offset in $\Gamma$, perhaps due to anharmonicity in the trapping potential. As all spectra in the main text were taken with $t_< = 200\,\mathrm{ms}$, this measurement establishes the lower bound for any measurement of $\Gamma$ in the main text to be $\Gamma_\mathrm{F} = 18(3)\,\mathrm{s}^{-1}$.

## S2. PROPERTIES OF CONDUCTIVITY

### A. Calorimetry and Joule's Law observation

The temperatures of the samples are fit using a quantum Monte Carlo calculation of the equation of state of the Hubbard model (HM). The core of our calculation is based on source code from the U.C. Davis Quantum Electron Simulation Toolbox [S6], run on a cubic lattice with $4\times4\times4$ sites, nearest-neighbor hopping, and on-site interactions. We start by calculating a table of the density $\rho = \rho\,(T,\mu)$, doublon density $\rho_d = \rho_d\,(T,\mu)$, and average energy per site $\overline{E}(T,\mu)$ for a range of temperatures $T$ and chemical potentials $\mu$. Data is fit using a parity-projected density, $\rho_f = \rho - 2\rho_d$, and a spatially varying chemical potential $\mu(\boldsymbol{r}) = \mu_0 - V(\boldsymbol{r})$, where $V(\boldsymbol{r})$ is the harmonic trapping potential, and $\mu_0$ is the peak chemical potential. Thus, the calculation gives the anticipated observed filling $\rho_f(\boldsymbol{r})$ as a function of thermodynamic fit parameters $T$ and $\mu_0$, along with calculated HM parameters $t$ and $U$.

Unlike our prior work [S7], four planes near the center of the trap are selected, and the quantum gas microscope is not used in single-atom-counting mode. Instead, the number of counts per atom (typically 1500) is an additional fit parameter for each image. A radial average is taken, to create a data set as shown in Fig. S3. The nearest-neighbor hopping rate $t$ and the on-site interaction strength $U$ are calculated from single-band Wannier functions; lattice depth is calibrated with amplitude modulation spectroscopy. Depths of the lattice in each direction are tuned to be equal within error ($0.1\,E_R$).

The calorimetry procedure may also be used as a complementary means to quantify the conductivity. Heat deposition into the sample through driving is an unavoidable effect, since a finite real conductivity signifies a dissipative response. The energy absorption rate $r_\mathrm{EA}$ may be measured, and follows a form of Joule's Law for neutral atoms with external forcing [S5, S8],

$$\mathrm{Re}\left[\sigma_{xx}(\omega)\right] = 2\frac{r_{EA}}{|F_x|^2}\,, \tag{S2}$$

Specifically, the energy absorption rate $r_{EA}$ is here measured by a sequence of thermometry measurements with variable driving times $t_d$. For each drive frequency $\omega$, images are taken and fit for five different $t_d$, up to $1000\,\mathrm{ms}$. Using the best-fit $T$ and $\mu_0$, the total energy of the system is calculated using the local density approximation: $E_\mathrm{tot} = \sum_{\boldsymbol{r}} \left\{\overline{E}\,[T,\mu(\boldsymbol{r})] + \rho\,[T,\mu(\boldsymbol{r})]\,V(\boldsymbol{r})\right\}$, summing over the positions $\boldsymbol{r}$ of sites in a $80\times80\times20$ lattice, where $\overline{E}$

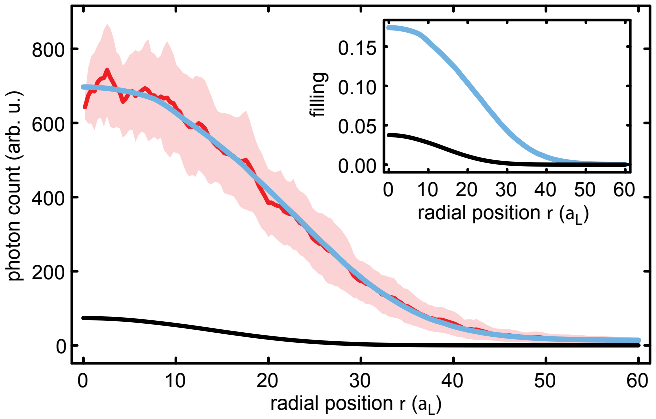


FIG. S3. **Example of thermometry**. The intensity distribution of in-situ fluorescence is used to determine number and temperature of the ultracold sample, as described in the text. Here, the observed photon counts and statistical uncertainty are shown versus radius as a red line and band. The blue line is the fitted parity-projected density; the black line is the doublon density. (Inset:) Calculated filling, without parity projection (blue line), and doublon density (black line) now shown on a calibrated vertical scale.

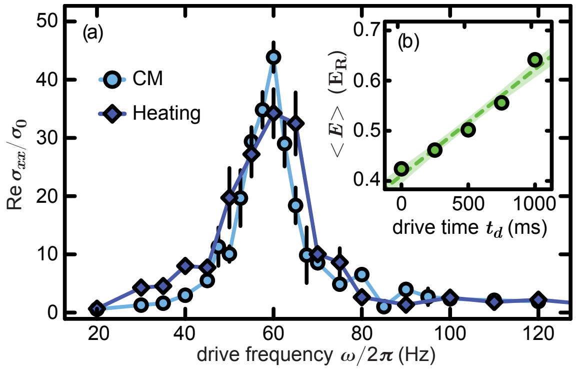


FIG. S4. **Joule's Law.** (a) The real on-axis conductivity Re$[\sigma_{xx}]$ determined by two independent methods are compared versus drive frequency. Purple points (♦) show Re$[\sigma_{xx}]$ determined from Eq. (S2) and the rate of energy absorption across $t_d = 0\,\mathrm{ms} - 1000\,\mathrm{ms}$; blue points (○) show Re$[\sigma_{xx}]$ determined as in the main text, from c.m. dynamics at $t_d = 0\,\mathrm{ms} - 100\,\mathrm{ms}$. The two methods show qualitative agreement. Conditions are $V = 2.5E_R$ and background scattering length. Lines are provided as a guide to the eye. (b) Example at 70 Hz drive frequency of energy absorption versus drive time. The slope (fit shown as a dashed line) is a measure of Re$[\sigma_{xx}]$ through Joule's Law.

is the qmc-calculated average energy per site with $T$ and local $\mu(\boldsymbol{r})$. $r_{EA}$ is determined by a linear fit to $E_{\mathrm{tot}}(t)$ at each drive frequency, from the linear increase in average energy with respect to time, as illustrated in Figure S4(b).

Figure S4(a) shows the Re$[\sigma_{xx}]$ determined from $r_{EA}$, and compares it with the Re$[\sigma_{xx}]$ as determined from the centre-of-mass response. The two methods show excellent agreement, with a best-fit correlation of 0.9(1). Differences are due the longer drive time for the $r_{EA}$ method, and systematic errors in calorimetry. The on-resonant heating rate was sufficient to double the temperature in $\sim$1 s, and conductivity is reduced at higher temperature. For delicate lower-temperature phases, an optimal measurement strategy might gather signal off-peak, for instance by probing Im$[\sigma]$ and using Kramers-Kronig relations.

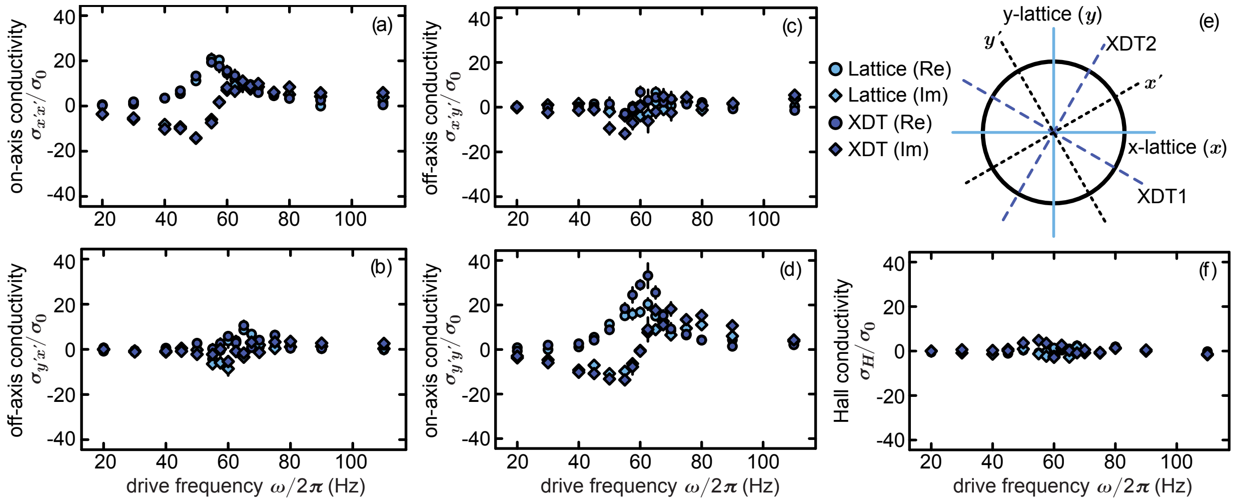


FIG. S5. **Tensor nature of conductivity.** The conductivity tensor is determined by measuring response when forcing along the lattice axes $(x, y)$, and comparing to when forcing along the XDT axes, which differ by an angle of $\pi/6$. (a-d) The full conductivity tensor, reported in the basis $(x', y')$. On-diagonal terms shown in (a) and (d) are more prominent than off-diagonals in (b) and (c). (e) Axes used for forcing in the two sets of measurements are shown (blue, solid) and (purple, dashed). The tensors are expressed in a common (black, dotted) basis. (f) Hall conductivity $\sigma_H/\sigma_0$ is within experimental fluctuation of zero, as expected. All data shown here is for depth $V = 2.5E_R$, $U/t_0 = 0.7$.

### B. Tensor response

Our experimental protocol allows us to provide a force to the sample along any axis. Choosing any two non-collinear axes enables the determination of the two-dimensional conductivity tensor $\sigma_{\alpha\beta}(\omega)$ describing transport in a plane. Knowledge of the tensor $\sigma_{\alpha\beta}(\omega)$ is of interest because it reveals spatial and temporal symmetries of the sample.

Figure S5(a-d) shows the conductivity tensor determined through two different choices of pairs of forcing axes: either along the axes of the in-plane optical lattices, or along the axes of the XDT beams, which are rotated by $\pi/6$ from the lattice axes [see Fig.S5(e)]. We find that the components of the conductivity tensors obtained through two different choices of pairs of measurement axes possess similar values when recast into a common basis ($x', y'$ as shown).

At each frequency, one can decompose $\sigma_{\alpha\beta}$ into its symmetric and anti-symmetric parts, $\sigma_{\alpha\beta} = \sigma_{\alpha\beta}^{(\mathrm{S})} + \sigma_{\alpha\beta}^{(\mathrm{A})}$. The symmetric conductivity is decomposed into the sum of its real and imaginary parts which are fully characterized by their eigenvalues and the rotation angle for which they are diagonal. In this case, due to the near isotropy of the system, eigenvalues are nearly degenerate and such a rotation angle is ill-defined. The anti-symmetric $\sigma_{\alpha\beta}^{(\mathrm{A})}$ has only one scalar degree of freedom (in two dimensions), which is the Hall conductivity,

$$\sigma_H = \frac{\sigma_{\alpha\beta} - \sigma_{\beta\alpha}}{2}. \tag{S3}$$

and which is invariant under rotation. In Fig. S5(f), we allow for the possibility that an anti-symmetric part of the conductivity tensor exists, and plot its determined value within the frequency band of interest. As expected for our system, $\sigma_H$ is consistent with zero: there is no broken time-reversal symmetry in the Hamiltonian. This can be further quantified using a sum rule for the off-diagonal conductivity. Defining the Hall angle as $\tan\theta_H = \sigma_H/\sigma_{xx}$ [S9] , then

$$\frac{2}{\pi}\int_0^\infty d\omega\, \mathrm{Re}\tan\theta_H = \omega_H \tag{S4}$$

where $\omega_H$ is the Hall frequency, which is unaffected by interactions, and is also the cyclotron frequency $eB/m$ for a free electron. From our data we find $\omega_H = 2\pi \times (0 \pm 2)\,\mathrm{Hz}$, consistent with zero. Despite the null result of this measurement, it provides a tool to explore Hall physics, and an alternative to previously demonstrated methods [S10–S13].

## S3. EIGENSPECTRUM FOR LATTICE PLUS PARABOLIC POTENTIAL

Following [S14, S15], we consider eigenstates $|\Phi^n\rangle$ of the single-band lattice plus parabolic potential to be comprised of a sum of ground-band Wannier functions:

$$\Phi^n(x,t) = \sum_j z_j^n(t) w_0(x - j a_L) \tag{S5}$$

where $z_j^n(t)$ gives the time-dependent amplitude of the Wannier function on the $j$th site, for the $n$th eigenstate of the system. In the tight-binding approximation, for a non-interacting system, separation of the Schroedinger equation yields solutions of the form:

$$z_j^n(t) = c_j^n e^{-iE_n t/\hbar} \tag{S6}$$

$$E_n c_j^n = -t(c_{j+1}^n + c_{j-1}^n) + V_P j^2 c_j^n \tag{S7}$$

where $V_P = m\omega_0^2 a_L^2/2$ describes the strength of the harmonic trapping potential. This recursion relation is may be recast into a momentum basis, through definition of the $\pi$-periodic functions $\psi_n(\xi) = \sum_j c_j^n e^{2ij\xi}$. Then, one obtains the following differential equation for $\psi_n(\xi)$:

$$E_n\psi_n(\xi) = -2t\cos(2\xi)\psi_n(\xi) - \frac{V_P}{4}\frac{\partial^2}{\partial\xi^2}\psi_n(\xi) \tag{S8}$$

Defining the parameter $q = 4t/V_P$, this may be put in the form of a Mathieu differential equation, with known eigenvalues and eigenstates:

$$E_{2r} = \frac{V_P}{4} a_{2r}(q) \qquad E_{2r+1} = \frac{V_P}{4} b_{2r}(q) \tag{S9}$$

$$\psi_{2r}(\xi) = \mathrm{ce}_{2r}(\xi; q) \qquad \psi_{2r+1}(\xi) = \mathrm{se}_{2r}(\xi; q) \tag{S10}$$

where $\text{ce}(\xi;q)$ and $\text{se}(\xi;q)$ are even and odd Mathieu functions, respectively, and $a_{2r}(q)$ and $b_{2r}(q)$ are their respective characteristic values.

This representation of the eigenproblem maps the dynamics in the lattice onto that of a one-dimensional particle with periodic boundary conditions. Defining the coordinate $\xi \in [-\pi/2, \pi/2]$ and its conjugate momentum $P_\xi = -i\hbar\partial_\xi$, Eq. (S8) can be recast as

$$H_{\text{eff}}\psi_n = E_n\psi_n \tag{S11}$$

with the effective Hamiltonian $H_{\text{eff}} = -2t\cos(2\xi) + V_P P_\xi^2/4\hbar^2$. This formal analogy allows us to readily calculate the thermodynamical properties of an ensemble of non-interacting particles trapped in a lattice plus harmonic potential. Indeed, in the quasi-classical limit (for characteristic energies larger than the level spacing) a sum over eigenstates can be replaced by a sum over the classical phase-space $(\xi, P_\xi)$. As an example, the partition function of Boltzmann particles is given by

$$Z \simeq \int \frac{d\xi dP_\xi}{2\pi\hbar} e^{-\beta(-2t\cos(2\xi)+V_P P_\xi^2/4\hbar^2)} = \sqrt{\frac{\pi k_B T}{V_P}} I_0(2\beta t), \tag{S12}$$

where $I_0$ is the zeroth order modified Bessel function of the first kind. The eigenspectrum provided by such a solution only applies in the tight-binding approximation. The spacing of the lowest energy eigenstates, which dominate the observed resonances in the conductivity spectrum, have energetic spacing $\hbar\omega_0^* = V_P\sqrt{q} = \hbar\omega_0\sqrt{m/m_0^*}$, which diverges as the lattice depth $V \to 0$. To correct this, the effects of next-nearest (n.n.) and next-next-nearest (n.n.n.) neighbor tunneling were considered. These tunneling terms modify the recursion relation in Eq. (S6) to become

$$E_n c_j^n = -t''(c_{j+3}^n + c_{j-3}^n) - t'(c_{j+2}^n + c_{j-2}^n) - t(c_{j+1}^n + c_{j-1}^n) + V_P j^2 c_j^n \tag{S13}$$

where $t'$ and $t''$ are the n.n. and n.n.n. tunneling coefficients. Proceeding as before, in the frequency basis:

$$E_n\psi_n(\xi) = 2t''\cos(6\xi)\psi_n(\xi) + 2t'\cos(4\xi)\psi_n(\xi) + 2t\cos(2\xi)\psi_n(\xi) - \frac{V_P}{4}\frac{\partial^2}{\partial\xi^2}\psi_n(\xi) \tag{S14}$$

This is an example of a Hill differential equation, and is difficult to solve in general. We instead treat the higher order tunneling terms as a perturbation to the frequency-space representation of the Hamiltonian:

$$H' = 2t''\cos(6\xi) + 2t'\cos(4\xi) \tag{S15}$$

Then, the corrected eigenspectrum to 1st order may be calculated from the known solutions to the Mathieu ODE as:

$$E_n' = E_n + \langle\psi_n|H'|\psi_n\rangle \tag{S16}$$

Including such a perturbation gives the correct frequency splitting for the lowest energy states.

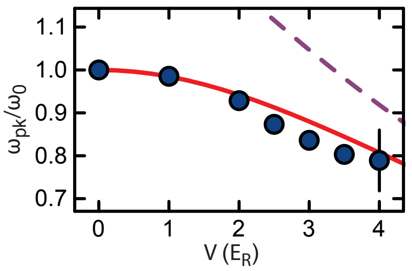


FIG. S6. The peak frequency $\omega_{\text{pk}}/\omega_0$ renomalization, compared to the exact $(m_{xx}^*(0)/m)^{-1/2}$ (solid line) and tight-binding $(m_0^*/m)^{-1/2}$ (dashed) at $q = 0$.

Figure S6 shows the necessity of the corrections for our data. For weak interactions, the peak response frequency $\omega_{\text{pk}}$ will be at the nearly uniform spacing between levels in the harmonic part of the spectrum. The figure compares $\omega_{\text{pk}}$ to the TB prediction and to the beyond-TB correction described above.

## S4. F-SUM IN CONTINUUM AND SINGLE-BAND HUBBARD MODELS

In this section, we calculate the f-sum

$$S_{\alpha\beta}^{\infty} = \frac{2}{\pi}\int_0^\infty d\omega\, \text{Re}\,\sigma_{\alpha\beta} = \frac{N^2}{\hbar^2}\left\langle [\hat{R}_\alpha, [\hat{H}, \hat{R}_\beta]] \right\rangle = \frac{N}{i\hbar}\left\langle \left[\hat{R}_\alpha, \hat{J}_\beta\right] \right\rangle \tag{S17}$$

and show how introducing a natural energy cut-off via the single-band Hubbard model relates to experimental results.

### A. Continuum

Before treating the HM, we evaluate the f-sum for a continuous space under the condition that the potential energy depends only on position. As physical systems exist in continuum, this is the result that is obtained for any physical Hamiltonian when considering all frequencies and eigenstates. For N interacting particles in a trap or in free space,

$$\hat{H} = \sum_{i}^{N} \frac{1}{2m}(\hat{p}_{x,i}^2 + \hat{p}_{y,i}^2 + \hat{p}_{z,i}^2) + V(\hat{\boldsymbol{r}}_1, \hat{\boldsymbol{r}}_2, \ldots, \hat{\boldsymbol{r}}_N) \tag{S18}$$

The center-of-mass operator along the $\beta = x$ direction,

$$\hat{R}_x = \frac{1}{N}\sum_i \hat{x}_i, \tag{S19}$$

commutes with all terms in the Hamiltonian except for those containing momentum terms $\hat{p}_x$, therefore

$$[\hat{H}, \hat{R}_x] = \frac{1}{2mN}\sum_{j,i}[\hat{p}_{x,i}^2, \hat{x}_i] = \frac{i\hbar}{mN}\sum_j \hat{p}_{x,j} \tag{S20}$$

$$\text{or} \quad \hat{J}_\beta = N\frac{d\hat{R}_\beta}{dt} = \frac{iN}{\hbar}[\hat{H}, \hat{R}_\beta] = \sum_j \frac{\hat{p}_{\beta,j}}{m} \tag{S21}$$

The latter relation shows that the current comes simply from the momentum of each particle, in free space. The commutator in the f-sum Eq. (S17) is

$$[\hat{R}_\alpha, [\hat{H}, \hat{R}_\beta]] = \frac{i\hbar}{mN^2}\sum_{j,i}[\hat{r}_{\beta,i}, \hat{p}_{\alpha,j}] = \frac{\hbar^2}{mN}\delta_{\alpha\beta} \tag{S22}$$

Therefore, the f-sum evaluates to

$$S_{\alpha\beta}^{\infty} = \frac{2}{\pi}\int_0^\infty d\omega \, \mathrm{Re}\, \sigma_{\alpha\beta} = \frac{N}{m}\delta_{\alpha,\beta} \tag{S23}$$

where this result is independent of temperature, interaction strength, or trapping potential. The result is diagonal: the f-sum will be zero for off-diagonal elements of the conductivity tensor, which measure response orthogonal to the drive direction.

### B. f-sum in the Hubbard model

The Hubbard Hamiltonian for spin-half fermions is

$$\hat{H} = \underbrace{-t\sum_{\langle j,k\rangle,s} \hat{c}_{j,s}^\dagger \hat{c}_{k,s}}_{\hat{H}_0} + \underbrace{U\sum_\ell \hat{n}_{\ell\uparrow}\hat{n}_{\ell\downarrow}}_{\hat{H}_U} + \underbrace{\frac{m}{2}\sum_\ell(\omega_x^2 x_\ell^2 + \omega_y^2 y_\ell^2 + \omega_z^2 z_\ell^2)(\hat{n}_{\ell\uparrow} + \hat{n}_{\ell\downarrow})}_{\hat{V}_{\mathrm{HO}}} \underbrace{- \mu_\uparrow \sum_\ell \hat{n}_{\ell\uparrow} - \mu_\downarrow \sum_\ell \hat{n}_{\ell\downarrow}}_{-\mu_\uparrow \hat{N}_\uparrow - \mu_\downarrow \hat{N}_\downarrow} \tag{S24}$$

where $t$ is the hopping energy between adjacent sites, $\langle j,k\rangle$ are nearest-neighbors connected by tunneling, $U$ is the on-site interaction energy, and $\mu_s$ is the chemical potential for spin-$s$. $\hat{c}_{\ell,s}^\dagger$ is the operator that creates an atom of spin $s$ on site index $\ell$ located at $(x_\ell, y_\ell, z_\ell)$, and $\hat{n}_{\ell,s} = \hat{c}_{\ell,s}^\dagger \hat{c}_{\ell,s}$ is the number operator. We use a spin-half basis, where $s$ can be $\uparrow$ or $\downarrow$, and only unlike spins interact. The $\hat{n}_{\ell\uparrow}\hat{n}_{\ell\downarrow}$ term written out in field operators is normally ordered, as $\hat{c}_{\ell\uparrow}^\dagger \hat{c}_{\ell\downarrow}^\dagger \hat{c}_{\ell\uparrow}\hat{c}_{\ell\downarrow}$.

In the lattice, the c.m. position operator is

$$\hat{R}_\alpha = \frac{1}{N}\sum_\ell r_{\alpha,\ell}(\hat{n}_{\ell\uparrow} + \hat{n}_{\ell\downarrow}) \tag{S25}$$

where $r_{\alpha,\ell}$ is the position along direction $\alpha$ of the site $\ell$. Since position operators commute, $[\hat{H}_U, \hat{R}_\alpha] = 0$, $[\hat{V}_{\mathrm{HO}}, \hat{R}_\alpha] = 0$, and $[\mu\hat{N}, \hat{R}_\alpha] = 0$. Just like for particles in free space, it is only the kinetic energy term $\hat{H}_0$ that contributes to the current, or to the f-sum (see Sec. S4 B).

The global current operator is then

$$\hat{J}_\beta = \frac{iN}{\hbar}[\hat{H}_0, \hat{R}_\beta] = \frac{-it}{\hbar} \sum_{\langle j,k\rangle,s} (r_{\beta,k} - r_{\beta,j})\hat{c}^\dagger_{j,s}\hat{c}_{k,s} \,. \tag{S26}$$

This can be generalized beyond tight binding by taking $t$ into the sum as $t_{j,k}$, and allowing tunneling between any sites $j, k$ that are not-necessarily nearest neighbors.

Using Eqs. (S17), (S25), and (S26), and including beyond tight-binding terms, the f-sum of the HM is:

$$\begin{aligned} S_{\alpha\beta} &= \frac{N}{i\hbar}\left\langle \left[\hat{R}_\alpha, \hat{J}_\beta\right]\right\rangle \\ &= -\frac{1}{\hbar^2}\left\langle \left[\sum_\ell r_{\alpha,\ell}\hat{n}_\ell, \sum_{j,k} t_{j,k}(r_{\beta,k} - r_{\beta,j})\hat{c}^\dagger_j\hat{c}_k\right]\right\rangle \\ &= -\frac{1}{\hbar^2}\sum_{j,k} t_{j,k}(r_{\alpha,j} - r_{\alpha,k})(r_{\beta,k} - r_{\beta,j})\left\langle \hat{c}^\dagger_j\hat{c}_k\right\rangle \end{aligned} \tag{S27}$$

where $\alpha$ and $\beta$ are arbitrary directions. In the case where $\alpha$ and $\beta$ are co-aligned to any one axis of the cubic lattice, and there is only nearest-neighbor hopping, this takes a simple form,

$$S_{xx} = -\frac{a_L^2}{\hbar^2}\left\langle \hat{H}_{0x}\right\rangle \tag{S28}$$

However when all lattice directions are symmetric, this is true for any direction. In general, for an isotropic, $d$-dimensional, separable lattice in tight binding,

$$S_{\alpha\alpha} = -\frac{a_L^2}{\hbar^2}\frac{E_K}{d} \tag{S29}$$

where $E_K = d\left\langle \hat{H}_{0x}\right\rangle$ is the kinetic energy.

The single-band HM does *not* satisfy Eq. (S23), since the higher bands are required for a complete set of eigenstates. It describes the low-frequency excitations of a system, capturing a partial f-sum. We can write it in the form of $N/m$ nonetheless, but with an inverse "band mass" replacing the inverse bare mass

$$\frac{1}{m_{\text{band}}} \equiv \left\langle \frac{1}{m^*_{\alpha\alpha}}\right\rangle = \frac{S_{\alpha\alpha}}{N} \tag{S30}$$

The rationale for this is explained further in the next section.

### C. Relation of f-sum to effective mass

For a uniform lattice, there is an alternative perspective on the f-sum Eq. (S27), relating it to the expectation value of the effective mass. For a particular Bloch vector $|\boldsymbol{k}\rangle$, the effective mass tensor is

$$\frac{1}{m^*_{\alpha\beta}(\boldsymbol{k})} \equiv \frac{1}{\hbar^2}\frac{\partial^2\epsilon(\boldsymbol{k})}{\partial k_\alpha \partial k_\beta} \tag{S31}$$

where $\epsilon(\boldsymbol{k}) = \langle \boldsymbol{k}\,|\,\hat{H}_0\,|\,\boldsymbol{k}\rangle$. For an isotropic lattice with any range of hopping,

$$\epsilon(\boldsymbol{k}) = -\frac{1}{M}\sum_{j,k} t_{j,k}e^{-i\boldsymbol{k}\cdot(\boldsymbol{r}_j - \boldsymbol{r}_k)} \tag{S32}$$

where $M$ is the number of sites. Since $\partial_{k_\alpha}e^{-i\boldsymbol{k}\cdot\boldsymbol{r}_j} = -ir_{\alpha,j}e^{-i\boldsymbol{k}\cdot\boldsymbol{r}_j}$, the effective mass is

$$\frac{1}{m^*_{\alpha\beta}(\boldsymbol{k})} = \frac{1}{\hbar^2 M}\sum_{j,k} t_{j,k}(r_{\alpha,j} - r_{\alpha,k})(r_{\beta,j} - r_{\beta,k})e^{-i\boldsymbol{k}\cdot(\boldsymbol{r}_j - \boldsymbol{r}_k)} \tag{S33}$$

The relation to the f-sum in Eq. (S27) can be found by expressing $\langle \hat{c}_j^\dagger \hat{c}_k \rangle$ in terms of momentum occupation:

$$\langle \hat{c}_j^\dagger \hat{c}_k \rangle = \frac{1}{M} \sum_{\boldsymbol{k},\boldsymbol{k'}} e^{-i\boldsymbol{k}\cdot\boldsymbol{r}_j + i\boldsymbol{k'}\cdot\boldsymbol{r}_k} \langle \hat{c}_{\boldsymbol{k}}^\dagger \hat{c}_{\boldsymbol{k'}} \rangle \tag{S34}$$

For thermal equilibrium, $\langle \hat{c}_{\boldsymbol{k}}^\dagger \hat{c}_{\boldsymbol{k'}} \rangle = f_{\boldsymbol{k}} \delta_{\boldsymbol{k},\boldsymbol{k'}}$, where $f_{\boldsymbol{k}}$ are thermal weights that satisfy $\sum f_{\boldsymbol{k}} = N$. Using these relations in Eq. (S27), we find

$$\begin{aligned} S_{\alpha\beta} &= -\frac{1}{\hbar^2} \sum_{j,k} t_{j,k} (r_{\alpha,j} - r_{\alpha,k})(r_{\beta,k} - r_{\beta,j}) \langle \hat{c}_j^\dagger \hat{c}_k \rangle \\ &= \sum_{\boldsymbol{k}} f_{\boldsymbol{k}} \frac{1}{\hbar^2 M} \sum_{j,k} t_{j,k} (r_{\alpha,j} - r_{\alpha,k})(r_{\beta,j} - r_{\beta,k}) e^{-i\boldsymbol{k}\cdot(\boldsymbol{r}_j - \boldsymbol{r}_k)} \\ &= \sum_{\boldsymbol{k}} f_{\boldsymbol{k}} \frac{1}{m^*_{\alpha\beta}(\boldsymbol{k})} = N \left\langle \frac{1}{m^*_{\alpha\beta}} \right\rangle \end{aligned} \tag{S35}$$

This is a more general expression than Eq. (S29), and applies to non-separable lattices for instance. From this derivation, we see the rationale of defining the band mass through Eq. (S30). In the isotropic, tight-binding, Maxwell-Boltzmann case, where the fugacity is $z_\uparrow = n_\uparrow I_0(2\beta t)^{-d}$ in $d$ dimensions, and $n_\uparrow$ is the filling per spin state,

$$\left\langle \frac{1}{m^*_{xx}} \right\rangle = \frac{1}{m^*_0} \frac{I_1(2\beta t)}{I_0(2\beta t)} \tag{S36}$$

where $I_0$ and $I_1$ are modified Bessel functions of the first kind, and $m^*_0$ is the tight-binding effective mass at $q = 0$, i.e. $m/m^*_0 = \pi^2 t/E_R$.

### D. Effect of the harmonic trap

As was argued in Sec. S4 B, because the c.m. position operator commutes with the harmonic trap operator ($[\hat{V}_{\text{HO}}, \hat{R}_\alpha] = 0$), the f-sum may still be evaluated using Eq. (S27), or Eq. (S28) in the isotropic, tight-binding case. Despite the fact that the f-sum still depends only on the kinetic energy of the system, $\langle \hat{H}_{0x} \rangle$, it is important to ascertain whether the trap modifies the expectation value of this operator.

The trap modifies the expected f-sum only slightly, as shown in Fig. S7, and only in the limit where temperature is less than the energetic splitting of the eigenstates, $k_B T/\hbar\omega^*_0 < 1$, where $\omega^*_0$ is the dressed trap frequency. This can be understood using the semiclassical approximation and Maxwell-Boltzmann statistics, and application of the Hellmann-Feynman Theorem.

Take the non-interacting limit of the Hubbard Hamiltonian given in Eq S24. Suppose it has eigenstates $|\psi_\alpha\rangle$, with eigenenergies $E_\alpha$. Then, the partition function in thermal equilibrium is

$$Z = \sum_\alpha e^{-\beta E_\alpha} \tag{S37}$$

and its derivative with respect to the tunneling energy in the Hamiltonian is

$$\frac{\partial Z}{\partial t} = -\beta \sum_\alpha \frac{\partial E_\alpha}{\partial t} e^{-\beta E_\alpha} \tag{S38}$$

The Hellman-Feynman Theorem states that $\partial_t E_\alpha = \langle \psi_\alpha | \partial_t \hat{H} | \psi_\alpha \rangle$, which in this case reduces to $\partial_t E_\alpha = \langle \psi_\alpha | \hat{H}_{0x} | \psi_\alpha \rangle / t$, where $\hat{H}_{0x}$ is the kinetic energy operator. Therefore, the expectation value of kinetic energy may be calculated directly from the partition function, via

$$\beta \langle \hat{H}_{0x} \rangle = -N \frac{t}{Z} \frac{\partial Z}{\partial t} \,. \tag{S39}$$

In the semiclassical approximation, the partition function is given by Eq. (S12). Equation (S39) then evaluates to

$$\langle \hat{H}_{0x} \rangle = -2Nt\frac{I_1(2\beta t)}{I_0(2\beta t)} \tag{S40}$$

Using Eq. (S27), we find that

$$\frac{S_{xx}}{N} = \frac{2ta_L^2}{\hbar^2}\frac{I_1(2\beta t)}{I_0(2\beta t)} = \frac{1}{m_0^*}\frac{I_1(2\beta t)}{I_0(2\beta t)} \tag{S41}$$

which is exactly the same result as for the homogeneous lattice case considered in Sec. S4 C. This justifies the identification of the measured f-sums with a homogeneous lattice effective mass, despite the existence of the trap.

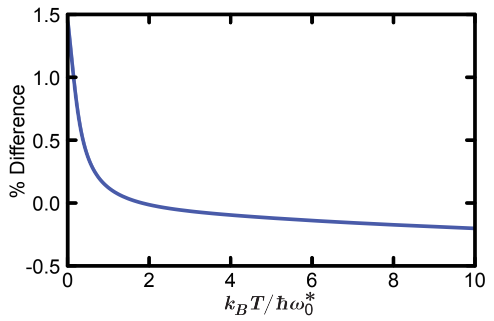


FIG. S7. **Effect of the trap on the f-sum**. The relative error between the f-sum calculated with or without a trap is compared versus temperature. As $T \to 0$, the error grows to $\sim 1.5\%$ for our harmonically-confined $2.5E_R$ lattice. Furthermore, the error is only appreciable for $k_BT/\hbar\omega_0^* < 1$, which is the scale of the spacing between harmonic oscillator energy levels.

The slight deviation in results appearing in Fig. S7 for $k_BT/\hbar\omega_0^* < 1$ may be understood in the context of momentum uncertainty associated with the harmonic confinement of the ground state of the system. Whereas in a homogeneous lattice system particles in the ground state may be fully delocalized, in the harmonically-confined system they are localized to within an oscillator length $a_{\mathrm{HO}}/\sqrt{2} = \sqrt{\hbar/m_{xx}^*(0)\omega_0^*}$. There is a corresponding uncertainty in quasi-momentum $\Delta k = 1/\sqrt{2}a_{\mathrm{HO}}$. At the bottom of the band, the uncertainty in energy is then:

$$\Delta E = \frac{\hbar^2}{2m_{xx}^*(0)}\left(\frac{1}{\sqrt{2}a_{\mathrm{HO}}}\right)^2 = \frac{1}{4}\hbar\omega_0^* \tag{S42}$$

This is half of the zero-point energy of the oscillator, which is precisely its contribution of kinetic energy to the ground state. Therefore, the expected shift in the f-sum is the ratio in this energy uncertainty and the expectation value for kinetic energy at the bottom of the band, or:

$$\Delta S_{xx} = \frac{\Delta E}{2t} = \frac{\hbar\omega_0^*}{8t} \tag{S43}$$

in tight-binding. For the $V = 2.5E_R$ lattice shown in Fig. S7, the expected shift is 1.6%, which agrees well with the full calculation.

## S5. KINETIC MODEL

The kinetic approach describes the dynamics of the system with a phase space distribution $f(\boldsymbol{r}, \boldsymbol{p})$ obeying the Boltzmann equation

$$\partial_t f + (\boldsymbol{F}_{\mathrm{trap}}(\boldsymbol{r}) + \boldsymbol{F}_{\mathrm{dr}}(t))\partial_{\boldsymbol{p}} f + \boldsymbol{v}\partial_{\boldsymbol{r}} f = I_{\mathrm{coll}}[f] \tag{S44}$$

where $\boldsymbol{F}_{\mathrm{trap}}$ is the trapping force, $\boldsymbol{F}_{\mathrm{dr}} = \boldsymbol{F}_0 \exp\{(i\omega t)\}$ is the driving force, and $I_{\mathrm{coll}}$ is the collisional integral, including blocking. We choose $f$ to be normalized as $\int d^3\boldsymbol{r}\, d^3\boldsymbol{p}\, f(\boldsymbol{r}, \boldsymbol{p}) = N$.

Assuming the cloud is weakly perturbed by the drive, we write $f = f^{(\mathrm{eq})} + f^{(\mathrm{dev})}$, with $f^{(\mathrm{dev})} \ll f^{(\mathrm{eq})}$, and $f^{(\mathrm{eq})}$ given by the stationary Boltzmann distribution: $I_{\mathrm{coll}}[f^{(\mathrm{eq})}] = 0$ and $\boldsymbol{F}_{\mathrm{trap}}(\boldsymbol{r})\partial_{\boldsymbol{p}} f^{(\mathrm{eq})} + \boldsymbol{v}\partial_{\boldsymbol{r}} f^{(\mathrm{eq})} = 0$. We can then write a linearized equation,

$$-i\omega f^{(\mathrm{dev})} + \boldsymbol{F}_{\mathrm{trap}}(\boldsymbol{r})\partial_{\boldsymbol{p}} f^{(\mathrm{dev})} + \boldsymbol{F}_0\partial_{\boldsymbol{p}} f^{(\mathrm{eq})} + \boldsymbol{v}\partial_{\boldsymbol{r}} f^{(\mathrm{dev})} = -\mathcal{L}[f^{(\mathrm{dev})}] \tag{S45}$$

where $\mathcal{L}$ is the linearized collision operator. This is formally solved as

$$f^{(\mathrm{dev})} = (i\omega - \mathcal{L} - \boldsymbol{F}_{\mathrm{trap}}(\boldsymbol{r})\partial_{\boldsymbol{p}} - \boldsymbol{v}\partial_{\boldsymbol{r}})^{-1}[\boldsymbol{F}_0\partial_{\boldsymbol{p}} f^{(\mathrm{eq})}] \tag{S46}$$

The global current is zero in equilibrium, so can be found solely from the displacement from equilibrium:

$$\boldsymbol{J}(t) = \int d^3\boldsymbol{r}\, d^3\boldsymbol{p}\, \boldsymbol{v} f^{(\mathrm{dev})}(\boldsymbol{r}, \boldsymbol{p}, t) \tag{S47}$$

### A. High-frequency limit

In this section, we discuss the high-frequency limit of conductivity. On grounds that current and force are purely real quantities, one can argue that the Laurent expansion of $\sigma$ should have even (odd) powers of $\omega$ in the real (imaginary) parts. Thus the leading order expansion is

$$\sigma(\omega) = \frac{i}{\omega}\left[S_1 - \frac{iS_2}{\omega} + \dots\right] \tag{S48}$$

One can show using Kramers-Kronig relations that $S_1 = \frac{1}{\pi}\int d\omega\ \mathrm{Re}\,\sigma$, the f-sum. In a Drude-form

$$\sigma = \frac{\sigma_0}{1 - i\omega\tau} \to i\frac{\sigma_0}{\omega\tau}\left[1 - \frac{i}{\omega\tau} + \dots\right] \tag{S49}$$

we see that $S_1 = \sigma_0/\tau$ and $\tau^{-1} = S_2/S_1$. In general, we expect $S_2$ to be extensive, and related to dissipation.

Equation (S46) can be expanded in the $\omega \to \infty$ limit as

$$f^{(\mathrm{dev})} = \frac{\boldsymbol{F}_0\partial_{\boldsymbol{p}} f^{(\mathrm{eq})}}{i\omega} - \frac{1}{\omega^2}(\mathcal{L} + \boldsymbol{F}_{\mathrm{trap}}(\boldsymbol{r})\partial_{\boldsymbol{p}} + \boldsymbol{v}\partial_{\boldsymbol{r}})[\boldsymbol{F}_0\partial_{\boldsymbol{p}} f^{(\mathrm{eq})}] \tag{S50}$$

Considering a drive along the $x$ direction,

$$\sigma_{xx} = \frac{1}{i\omega}\int d^3\boldsymbol{r}\, d^3\boldsymbol{p}\, v_x \partial_{p_x} f^{(\mathrm{eq})} - \frac{1}{\omega^2}\int d^3\boldsymbol{r}\, d^3\boldsymbol{p}\, v_x(\mathcal{L} + \boldsymbol{F}_{\mathrm{trap}}(\boldsymbol{r})\partial_{\boldsymbol{p}} + \boldsymbol{v}\partial_{\boldsymbol{r}})[\partial_{p_x} f^{(\mathrm{eq})}] + \dots \tag{S51}$$

We note that, via the product rule,

$$v_x(\boldsymbol{F}_{\mathrm{trap}}(\boldsymbol{r})\partial_{\boldsymbol{p}} + \boldsymbol{v}\partial_{\boldsymbol{r}})[\partial_{p_x} f^{(\mathrm{eq})}] = v_x\partial_{p_x}(\boldsymbol{F}_{\mathrm{trap}}(\boldsymbol{r})\partial_{\boldsymbol{p}} + \boldsymbol{v}\partial_{\boldsymbol{r}}) f^{(\mathrm{eq})} - v_x(\partial_{p_x}\boldsymbol{v})\partial_{\boldsymbol{r}} f^{(\mathrm{eq})}\,. \tag{S52}$$

Since $f^{(\mathrm{eq})}$ is the stationary phase-space density, the first term of the RHS vanishes. Furthermore, since the second term is a total derivative with respect to position, it cancels out when integrating over all space. Thus

$$\sigma_{xx} = \frac{1}{i\omega}\int d^3\boldsymbol{r}\, d^3\boldsymbol{p}\, v_x \partial_{p_x} f^{(\mathrm{eq})} - \frac{1}{\omega^2}\int d^3\boldsymbol{r}\, d^3\boldsymbol{p}\, v_x \mathcal{L}[\partial_{p_x} f^{(\mathrm{eq})}] + \dots \tag{S53}$$

We recover Eq. (S48) with

$$S_1 = -\int d^3\boldsymbol{r}\, d^3\boldsymbol{p}\, v_x \partial_{p_x} f^{(\mathrm{eq})} \tag{S54}$$

$$S_2 = -\int d^3\boldsymbol{r}\, d^3\boldsymbol{p}\, v_x \mathcal{L}[\partial_{p_x} f^{(\mathrm{eq})}] \tag{S55}$$

Integrating by parts Eq. (S54) and noting that for a single-particle dispersion relation $\epsilon(\boldsymbol{p})$, the velocity is defined by $v = \partial_{\boldsymbol{p}}\epsilon$, we have

$$S_1 = \int d^3\boldsymbol{r}\, d^3\boldsymbol{p}\, \frac{f^{(\mathrm{eq})}}{m^*_{xx}} \tag{S56}$$

where the effective mass is $1/m^*_{xx} = \partial^2_{p_x}\epsilon$. From this we recover the f-sum rule Eq. (S30).

In analogy with the Drude form, we define the effective damping rate $\tau^{-1} = S_2/S_1$. The definition coincides with the damping rate of a sudden momentum boost. Just after such an excitation, the distribution is shifted by $f^{(\mathrm{dev})} = -(\Delta p)\partial_{p_x} f^{(\mathrm{eq})}$, where $\Delta p$ is the change in momentum per particle due to the boost. The time derivative of the current afterwards is then

$$\dot{J}_x = \int d^3\boldsymbol{r}\, d^3\boldsymbol{p}\, v_x I_{\mathrm{coll}}[f] = \Delta p \int d^3\boldsymbol{r}\, d^3\boldsymbol{p}\, \mathcal{L}[\partial_{p_x} f^{(\mathrm{eq})}] = -\Delta p\, S_2. \tag{S57}$$

Since $J_x = \int d^3\boldsymbol{r}\, d^3\boldsymbol{p}\, v_x f^{(\mathrm{dev})} = \Delta p\, S_1$, we see that the current damping rate $-\dot{J}_x/J_x = S_2/S_1$, which is $\tau^{-1}$ as defined. (Section S5 C discusses the impulse response in a uniform lattice in more detail.)

The consequence of Eqs. (S54) and (S55) is that in a kinetic model, $S_1$ and $S_2$ are extensive quantities and take the general form $S_i = \int d^3\boldsymbol{r} s_i(\boldsymbol{r})$, with

$$s_1(\boldsymbol{r}) = \int d^3\boldsymbol{p}\, \frac{f^{(\mathrm{eq})}(\boldsymbol{r},\boldsymbol{p})}{m^*(\boldsymbol{p})} \tag{S58}$$

$$s_2(\boldsymbol{r}) = -\int d^3\boldsymbol{p}\, v_x \mathcal{L}[\partial_{p_x} f^{(\mathrm{eq})}] \tag{S59}$$

This property means that $S_1$ and $S_2$ for a trapped system can be obtained by integrating spatially the response of a uniform system. Physically, this comes from the fact that at high frequency, the amplitude of the driven motion is vanishingly small, such that over one oscillation cycle, the atoms at each position do not explore significant inhomogeneity. Finally, for a Boltzmann distribution, one can show that $S_2$ in a trap and in a homogenous system differ only by the geometric factor $\langle\rho\rangle/\rho_{\mathrm{hom}}$, where $\langle\rho\rangle$ is the density-weighted density.

### B. Collisional damping in a lattice

Based on the discussion of the previous section, we now neglect spatial variation, and consider collisional damping of a uniform lattice. We denote as $N_{\uparrow,\downarrow}$ for the number of atoms of each spin species, and $M = \prod_\alpha M_\alpha$ for the number of lattice sites, where $\alpha = \{x, y, z\}$ in three dimensions. In a cubic lattice, lattice sites are at $x_\ell = \ell a_L$, etc. We consider $J_\uparrow$ here, to be specific; but assume that $f = f_\uparrow = f_\downarrow$ throughout. The global current is $J = J_\uparrow + J_\downarrow$, with

$$\boldsymbol{J}_{\uparrow,\downarrow}(t) = \sum_{\boldsymbol{q}} \boldsymbol{v}(\boldsymbol{q}) f_{\uparrow,\downarrow}(\boldsymbol{q}, t)\,, \tag{S60}$$

where $v_\alpha(\boldsymbol{k}) = v_m \sin a_L k_\alpha = v_m \sin q_\alpha$, and $v_m = 2ta_L/\hbar$, in tight binding.

The collisional rate of relaxation of Bloch-state occupation for a particle in state 1 is given by:

$$\left.\frac{d}{dt}\right|_{\mathrm{coll}} f_1 = -\frac{2\pi}{\hbar}\frac{U^2}{M^2}\sum_{\boldsymbol{q}_2,\boldsymbol{q}_3}\{f_1 f_2(1-f_3)(1-f_4) - f_3 f_4(1-f_1)(1-f_2)\}\,\delta(E_{34}-E_{12}) \tag{S61}$$

The rate of change is zero when $f = f^{(\mathrm{eq})}$ has its equilibrium value. In Sec. S5 C we consider the impulse response, and in Sec. S5 D we evaluate the scattering integral numerically in the tight-binding limit.

### C. Impulse response

We consider the non-equilibrium distribution created by an external force $F_x$, which shifts quasi-momentum as $\hbar\dot{k}_x = F_x$, or $\dot{q}_x = (a_L/\hbar)F_x$. In the linear response regime, $\Delta q_x \ll \pi$, we show that both current and its damping are linear in $\Delta q_x$.

For a small displacement of the distribution from equilibrium, of the form [S16], the change may be expressed as

$$f^{(\mathrm{dev})} = f - f^{(\mathrm{eq})} = -\frac{\partial f^{(\mathrm{eq})}}{\partial E}\psi, \tag{S62}$$

where $\psi$ is some energetic displacement from equilibrium. Assuming that a small displacement $\Delta\boldsymbol{q}$ is resultant from an external force, we have

$$f^{(\mathrm{dev})} = -\Delta\boldsymbol{q}\cdot\frac{\partial f^{(\mathrm{eq})}}{\partial\boldsymbol{q}}. \tag{S63}$$

Since $f^{(\mathrm{eq})}$ is purely a function of $E$, then

$$\frac{\partial f^{(\mathrm{eq})}}{\partial\boldsymbol{q}} = \frac{df^{(\mathrm{eq})}}{dE}\frac{\partial E}{\partial\boldsymbol{q}} = \frac{df^{(\mathrm{eq})}}{dE}\frac{\hbar\boldsymbol{v}}{a_L}, \tag{S64}$$

which combined with the previous result shows

$$f^{(\mathrm{dev})} = -\frac{\hbar}{a_L}\Delta\boldsymbol{q}\cdot\boldsymbol{v}\frac{df^{(\mathrm{eq})}}{dE} \qquad \text{or} \qquad \psi(\boldsymbol{q},\Delta\boldsymbol{q}) = \frac{\hbar}{a_L}\Delta\boldsymbol{q}\cdot\boldsymbol{v}(\boldsymbol{q}). \tag{S65}$$

To evaluate Eq. (S61), it is useful to note that, to first order in $\psi$,

$$\sum_{2,3}\Big\{f_1f_2(1-f_3)(1-f_4)-f_3f_4(1-f_1)(1-f_2)\Big\}$$
$$= -\beta\sum_{2,3} f_1^{(\mathrm{eq})}f_2^{(\mathrm{eq})}(1-f_3^{(\mathrm{eq})})(1-f_4^{(\mathrm{eq})})\,(\psi_1+\psi_2-\psi_3-\psi_4)\ . \tag{S66}$$

Here we've used the fact that $\partial f^{(\mathrm{eq})}/\partial E = -\beta f^{(\mathrm{eq})}(1-f^{(\mathrm{eq})})$, and that the sum over any equilibrium combination of $f^{(\mathrm{eq})}$ must vanish.

In the case where the perturbation only focused on $x-$axis, the displacement in quasi-momentum is $\Delta k_x = \Delta q_x/a_L$ from equilibrium, and $\psi_x(\boldsymbol{q},\Delta q_x) = \hbar\Delta q_x v_x(\boldsymbol{q})/a_L$, so

$$\psi_1+\psi_2-\psi_3-\psi_4 = -(\hbar\Delta q_x/a_L)\Delta J_x(12;34), \tag{S67}$$

where $\Delta J_x(12;34) = v_x(\boldsymbol{q}_3)+v_x(\boldsymbol{q}_4)-v_x(\boldsymbol{q}_1)-v_x(\boldsymbol{q}_2)$ is the change in current from the collision process. Then Eq. (S61) simplifies to

$$\frac{d}{dt}\Big|_{\mathrm{coll}} f_1 = -\frac{2\pi}{\hbar}\frac{U^2}{M^2}\frac{\hbar\Delta q_x}{a_L}\beta\sum_{\boldsymbol{q}_2,\boldsymbol{q}_3}\Delta J_x(12;34)f_1^{(\mathrm{eq})}f_2^{(\mathrm{eq})}(1-f_3^{(\mathrm{eq})})(1-f_4^{(\mathrm{eq})})\,\delta(E_{34}-E_{12}). \tag{S68}$$

We see that only those collisions that result in a net change in current $\Delta J_x$ change the occupation.

Note that this displacement from equilibrium differs from that considered by Orso *et al.* [S17] due to a hydrodynamic displacement in velocity. In that case, $\psi$ is proportional to $\boldsymbol{\Delta v}\cdot\boldsymbol{q}$, so that $\psi_1+\psi_2-\psi_3-\psi_4$ is directly proportional to the net change in *quasi-momentum*, and normal collisions cause no change in distribution – only Umklapp collisions do not conserve $\boldsymbol{q}$. In contrast, conductivity measures the response to an external force, which continuously displaces quasi-momentum, and thus normal collisions do contribute to relaxation and to current damping outside of the hydrodynamic regime.

Next, we find the global current caused by the impulse $\Delta q_x$. Since $\langle \mathrm{J}_{\uparrow,\downarrow}\rangle = 0$ in equilibrium, we can replace $f_\uparrow$ by $f^{(\mathrm{dev})}$ in Eq. (S60). Taking the continuum limit of the sum, this is

$$\boldsymbol{J}_\uparrow(\Delta\boldsymbol{q}) = M\int f^{(\mathrm{dev})}\boldsymbol{v}(\boldsymbol{q})\,\frac{d\boldsymbol{q}}{(2\pi)^D} \tag{S69}$$

where

$$f^{(\mathrm{dev})}(E,\boldsymbol{q},\Delta\boldsymbol{q}) = \beta f^{(\mathrm{eq})}(E)(1-f^{(\mathrm{eq})}(E))\frac{\hbar}{a_L}\Delta\boldsymbol{q}\cdot\boldsymbol{v}(\boldsymbol{q}) \tag{S70}$$

and the Fermi-Dirac (FD) distribution is $f^{(\mathrm{eq})} = [1+z^{-1}\exp\{(\beta E_{\boldsymbol{q}})\}]^{-1}$. Choosing $\boldsymbol{\Delta q}$ to be along the $x$ lattice direction, the dot product isolates $v_x(q_x)$. Then the current is along $x$, i.e. $\boldsymbol{J}_\uparrow = \boldsymbol{u}_x J_\uparrow$, where

$$J_\uparrow(\Delta q_x) = \beta\frac{\hbar\Delta q_x}{a_L}M\int f^{(\mathrm{eq})}(\boldsymbol{q})(1-f^{(\mathrm{eq})}(\boldsymbol{q}))v_x^2(q_x)\,\frac{d\boldsymbol{q}}{(2\pi)^D} \tag{S71}$$

We see that the current response is linear in $\Delta q_x$. The intuitive interpretation is that $\hbar\Delta q_x/a_L$ is the impulse given by the external force. For a classical particle, the velocity response to an impulse is determined by the inverse mass. Implicitly defining the inverse band mass $\langle 1/m^*_{xx}\rangle$ in this way,

$$J_\uparrow(\Delta q_x) = N_\uparrow\langle v\rangle_{\Delta q_x} = N_\uparrow\frac{\hbar\Delta q_x}{a_L}\left\langle\frac{1}{m^*_{xx}}\right\rangle\ , \tag{S72}$$

we have

$$\left\langle\frac{1}{m^*_{xx}}\right\rangle = \frac{\beta}{n_\uparrow}\int f^{(\mathrm{eq})}(\boldsymbol{q})(1-f^{(\mathrm{eq})}(\boldsymbol{q}))v_x^2(q_x)\,\frac{d\boldsymbol{q}}{(2\pi)^D}\ , \tag{S73}$$

where $n_\uparrow$ is the filling per spin state, and can be obtained from $n_\uparrow = N_\uparrow/M = \int f^{(\mathrm{eq})}(\boldsymbol{q})d\boldsymbol{q}/(2\pi)^D$.

This intuitive result may be shown to be correct. For a particular $q_x$, the effective mass is $1/m^*_{xx}(q_x) = (a/\hbar)\partial v_x/\partial q_x$. Using:

$$\beta f^{(\mathrm{eq})}(\boldsymbol{q})(1-f^{(\mathrm{eq})}(\boldsymbol{q})) = -\frac{\partial f^{(\mathrm{eq})}}{\partial E} = -\frac{\partial f^{(\mathrm{eq})}}{\partial q_x}\frac{a_L}{\hbar v_x}\ , \tag{S74}$$

one factor of $v_x(q_x)$ cancels, so that

$$\left\langle \frac{1}{m^*_{xx}} \right\rangle = -\frac{a_L}{n_\uparrow \hbar} \int \frac{\partial f^{(\text{eq})}}{\partial q_x} v_x(q_x) \frac{d\boldsymbol{q}}{(2\pi)^D} = \frac{1}{n_\uparrow} \int f^{(\text{eq})} \frac{a_L}{\hbar} \frac{\partial v_x}{\partial q_x} \frac{d\boldsymbol{q}}{(2\pi)^D} = \frac{1}{n_\uparrow} \int f^{(\text{eq})} \frac{1}{m^*_{xx}(q_x)} \frac{d\boldsymbol{q}}{(2\pi)^D} \tag{S75}$$

where we have used integration by parts, and the fact that the two edges of the Brillouin zone are identical. In other words, the "band mass" gives the correct current response to a uniform $\Delta q_x$ kick across the thermally populated distribution, and thus the impulse response is proportional to the f-sum:

$$J(\Delta q_x) = \frac{\hbar \Delta q_x}{a_L} S_{xx} \tag{S76}$$

In the tight-binding, MB limit, this is

$$J_\uparrow(\Delta q_x) = N_\uparrow \frac{\hbar \Delta q_x}{a_L} \left\langle \frac{1}{m^*_{xx}} \right\rangle = \frac{N_\uparrow \hbar \Delta q_x}{a_L m^*_0} \frac{I_1(2\beta t)}{I_0(2\beta t)} \tag{S77}$$

### D. Scattering integral

The linear-response damping rate is $1/\tau = -(dJ/dt)/J$. Using Eqs. (S68) and (S76), the common pre-factor of $\hbar \Delta q_x / a_L$ cancels, leaving

$$\frac{1}{\tau} = \frac{2\pi\beta U^2}{\hbar N \langle 1/m^*_{xx} \rangle M^2} \sum_{\boldsymbol{q}_1, \boldsymbol{q}_2, \boldsymbol{q}_3} v_x(\boldsymbol{q}_1) \Delta J_x(12;34) f_1^{(\text{eq})} f_2^{(\text{eq})} (1 - f_3^{(\text{eq})})(1 - f_4^{(\text{eq})})\, \delta(E_{34} - E_{12}). \tag{S78}$$

Taking the continuum limit, $M^{-1} \sum_{\boldsymbol{q}} \to \prod_\alpha \{\int dq_\alpha / 2\pi\}$, where $\alpha$ indicates any of the $x$, $y$ and $z$ direction, the damping rate is

$$\frac{1}{\tau} = \frac{U^2}{\hbar t} \frac{2\pi\beta t M}{N \langle 1/m^*_{xx} \rangle} \left\{ \prod_\alpha \iiint \frac{dq_{1\alpha}}{2\pi} \frac{dq_{2\alpha}}{2\pi} \frac{dq_{3\alpha}}{2\pi} \right\} v_x(\boldsymbol{q}_1) \Delta J_x(12;34) f_1 f_2 (1 - f_3)(1 - f_4)\, \delta(E_{34} - E_{12}), \tag{S79}$$

where we drop the $^{(\text{eq})}$ specification on $f$ from here forward.

Now we simplify the expression in the tight-binding limit: both $v_x$ and $\Delta J_x$ are proportional to $v_m = 2ta_L/\hbar$; we can pull out a factor of $2t$ from the $\delta(E) = (2t)^{-1}\delta(E/2t)$; and note that the filling per spin state $n_\uparrow = N_\uparrow / M$. Thus, we obtain

$$\frac{\hbar \tau^{-1}}{U^2/t} = \frac{2\pi\beta t}{\int f \cos q_x \, d\boldsymbol{q}/(2\pi)^3} \times \left\{ \prod_{\alpha = x,y,z} \iiint \frac{dq_{1\alpha}}{2\pi} \frac{dq_{2\alpha}}{2\pi} \frac{dq_{3\alpha}}{2\pi} \right\} \frac{v_x(\boldsymbol{q}_1)}{v_m} \frac{\Delta J_x(12;34)}{v_m} f_1 f_2 (1 - f_3)(1 - f_4)\, \delta\left( \frac{E_{34} - E_{12}}{2t} \right). \tag{S80}$$

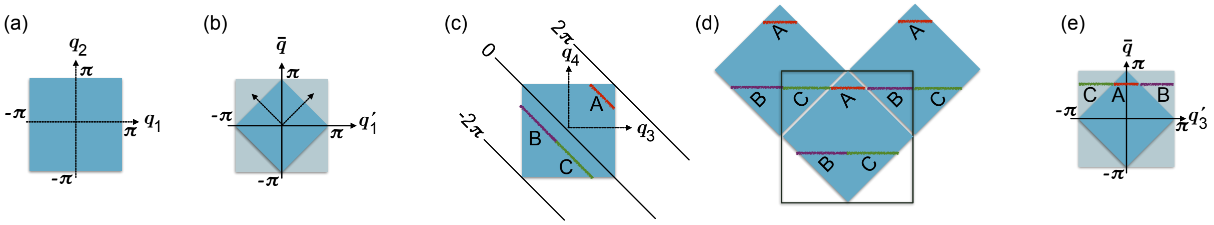


FIG. S8. **Allowed Quasi-momenta.** **(a)** Range of quasi-momentum along one axis for particles 1 and 2. **(b)** Range of $\bar{q}$ and $q_1'$: $\bar{q}$ is $-\pi \to \pi$, and the range of $q'$ is $-\pi + |\bar{q}| \to \pi - |\bar{q}|$. Note that the area is reduced by a factor of 2. **(c)** Total quasi-momentum is only conserved modulo $2\pi$. If events shown at A are allowed by strict $\delta(q)$ conservation, then events shown at B and C are also allowed: they are $\pm 1$ Umklapp events. **(d)** Showing adjacent (identical) zones, we see that events B and C can be considered to "wrap around" to the adjacent zones. **(e)** All valid final momenta, including these Umklapp events, can be captured without double counting by using the strict $\delta(q)$ to select A, and $\bar{q}$, but then allowing $q_3'$ to range from $-\pi \to \pi$.

To calculate the integral, we consider some transformations to the coordinates of quasi-momentum $q$. Since quasi-momentum is conserved (modulo $2\pi$) in elastic collisions, it is convenient to rewrite momenta in terms of the average (or shared) $\bar{\boldsymbol{q}} \equiv (\boldsymbol{q}_1 + \boldsymbol{q}_2)/2$ and a relative (or differential) as

$$\boldsymbol{q}_1' \equiv \boldsymbol{q}_1 - \bar{\boldsymbol{q}} \qquad \text{and} \qquad \boldsymbol{q}_2' \equiv \boldsymbol{q}_2 - \bar{\boldsymbol{q}}, \qquad \text{so that} \qquad \boldsymbol{q}_2' = -\boldsymbol{q}_1' \qquad \text{(relative momenta).} \tag{S81}$$

Functions of quasi-momentum are $2\pi$-periodic, and thus $q$ are only meaningful modulo $2\pi$. Let's now take the range of each $q_\alpha$ to be $-\pi$ to $+\pi$. Converting to the center-of-mass coordinates defined in Eq. (S81), one can show that the range of $\bar{q}$ is $-\pi \to \pi$, and the range of $q'$ is $-\pi + |\bar{q}| \to \pi - |\bar{q}|$. These are shown in Fig. S8(a,b). A subtlety comes when applying momentum conservation to the $q$. As discussed above, $q_4 = q_1 + q_2 - q_3$ *modulo* $2\pi$ in a collision, so that in each direction

$$q_{\alpha 1} + q_{\alpha 2} = q_{\alpha 3} + q_{\alpha 4} + 2\pi n$$

are allowed for $n = \pm 1$, Umklapp (UK) collisions, or $n = 0$, normal collisions. Figures S8(c,d,e) show that UK events are included simply by allowing the final relative momentum $q_3'$ to have the range $-\pi \to +\pi$, instead of $-\pi + |\bar{q}| \to \pi - |\bar{q}|$, and otherwise proceeding as if $q$ is strictly conserved.

Now we rewrite the $q$ integrals in center-of-mass coordinates, as discussed above. For each pair, such as $q_{1\alpha}$ and $q_{2\alpha}$, we write $\bar{q}_\alpha = (q_{1\alpha} + q_{2\alpha})/2$ and $q_\alpha' = q_{1\alpha} - \bar{q}_\alpha = (q_{1\alpha} - q_{2\alpha})/2$. One can show that

$$\iint_{-\pi}^{\pi} dq_1\, dq_2 \to 2\int_{-\pi}^{\pi} d\bar{q} \int_{-\pi+|\bar{q}|}^{\pi-|\bar{q}|} dq'. \tag{S82}$$

For the $q_3$ integral, strict conservation of momentum $\delta(q_4 + q_3 - q_1 - q_2)$ is $\frac{1}{2}\delta(\bar{q}_{34} - \bar{q}_{12})$, so that

$$\iint_{-\pi}^{\pi} dq_3\, dq_4 \delta(q_4 + q_3 - q_1 - q_2) \to 2\int_{-\pi}^{\pi} d\bar{q}_{34} \int_{-\pi+|\bar{q}|_{34}}^{\pi-|\bar{q}|_{34}} dq_3' \frac{1}{2}\delta(\bar{q}_{34} - \bar{q}_{12}) = \int_{-\pi+|\bar{q}|_{12}}^{\pi-|\bar{q}|_{12}} dq_3'. \tag{S83}$$

However as noted above, Umklapp events are included by extending the range of integration of $q_3'$ to $-\pi \to +\pi$, instead of $-\pi + |\bar{q}| \to \pi - |\bar{q}|$. Together, we have

$$\iiint \frac{dq_1}{2\pi}\frac{dq_2}{2\pi}\frac{dq_3}{2\pi} \to 2\int_{-\pi}^{\pi} \frac{d\bar{q}}{2\pi} \int_{-\pi+|\bar{q}|}^{\pi-|\bar{q}|} \frac{dq_1'}{2\pi} \int_{-\pi}^{\pi} \frac{dq_3'}{2\pi} \tag{S84}$$

for each direction. In center-of-mass coordinates, the currents and energies are

$$\begin{aligned} v_{x,1}/v_m &= \sin(\bar{q}_x + q_{x1}')\,, \\ \Delta J_x/v_m &= 2\sin\bar{q}_x\,(\cos q_{x3}' - \cos q_{x1}')\,, \\ \Delta\epsilon_\alpha &= \Delta E_\alpha/2t = -2\cos\bar{q}_\alpha\,(\cos q_{\alpha 3}' - \cos q_{\alpha 1}')\,. \end{aligned} \tag{S85}$$

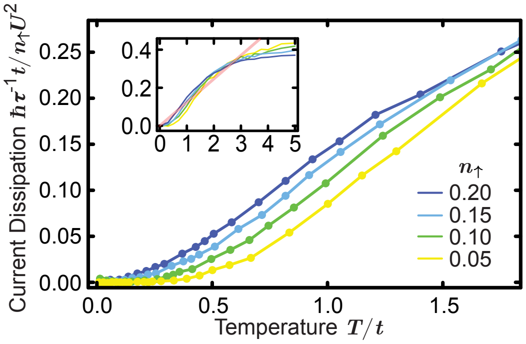


FIG. S9. **Current dissipation rate.** The collisional damping rate of current, scaled by $n_\uparrow U^2/\hbar t$, is shown versus temperature for various fillings. For the typical temperatures and densities explored in the data ($T > t$, $n_\uparrow < 0.2$), the damping rate scales almost linearly with filling, seen from the collapsing of calculations with different $n_\uparrow$. At lower temperature (where $\tau^{-1} \sim T^2$), blocking will play a role, and collisions will be blocked even with increased filling. In the inset, which shows a broader range of temperatures, the red line serves as a guide to the eye, illustrating range over which the calculated $\tau^{-1}/(nU^2/\hbar t)$ is approximately linear in temperature.

Therefore the main integral in Eq. (S80) is

$$\frac{\hbar\tau^{-1}}{U^2/t} = \frac{2\pi\beta t}{\int f \cos q_x \, d\boldsymbol{q}/(2\pi)^3} \left\{ 8 \prod_\alpha \int_{-\pi}^{\pi} \frac{d\bar{q}_\alpha}{2\pi} \int_{-\pi+|\bar{q}_\alpha|}^{\pi-|\bar{q}_\alpha|} \frac{dq'_{\alpha 1}}{2\pi} \int_{-\pi}^{\pi} \frac{dq'_{\alpha 3}}{2\pi} \right\}$$

$$\sin\left(\bar{q}_x + q'_{x1}\right) \, 2\sin\bar{q}_x \left(\cos q'_{x3} - \cos q'_{x1}\right) f_1 f_2 (1-f_3)(1-f_4)\, \delta \left[ -2 \sum_\alpha \cos\bar{q}_\alpha \left(\cos q'_{\alpha 3} - \cos q'_{\alpha 1}\right) \right]. \quad \text{(S86)}$$

Figure S9 shows results of numerical evaluation of this equation, for various fillings $n_\uparrow$ (fixed with chemical potential of the Fermi distribution) and temperatures $T/t = 1/\beta t$. The vertical axis is re-scaled by $n_\uparrow U^2/t$, which is a combination of the $U^2/t$ expected from the LHS of Eq. (S86), and an additional factor of filling. From the inset, we see that all curves cross around $T = 2t$. There is also an inflection between a low-temperature quadratic behavior (from blocking) and a high-temperature saturation (from an evenly filled band). The experimental temperatures are not low enough to see blocking, and thus Maxwell-Boltzmann statistics are a good approximation (although these plots, and the red theory curve in Fig. 3 of the main text, were calculated using Fermi-Dirac statistics).

Figure 3 in the main text uses $n_\uparrow U^2/t$ as the horizontal axis, with the measured damping rate $\Gamma$ as the vertical axis. The band of values (shown in red there) reflects the range of temperatures and chemical potentials used as inputs to the calculation, selected to match the range within the various data sets. The inset to Fig. 3 in the main text re-scales $\Gamma$ to dimensionless $\hbar\Gamma/T$. This gives a further tightening in the range of experimental predictions, since (as seen in the inset to Fig. S9), the scattering rate is approximately linear in $T$ in the experimental range $1 \lesssim T/t \lesssim 3$.

---


[S1] W. S. Bakr, J. I. Gillen, A. Peng, S. Foelling, and M. Greiner, "A quantum gas microscope for detecting single atoms in a Hubbard-regime optical lattice," Nature **462**, 74 (2009).

[S2] J. F. Sherson, C. Weitenberg, M. Endres, M. Cheneau, I. Bloch, and S. Kuhr, "Single-atom-resolved fluorescence imaging of an atomic Mott insulator," Nature **467**, 68 (2010).

[S3] A. Omran, M. Boll, T. A. Hilker, K. Kleinlein, G. Salomon, I. Bloch, and C. Gross, "Microscopic observation of pauli blocking in degenerate fermionic lattice gases," Phys. Rev. Lett. **115**, 263001 (2015).

[S4] D. Mitra, P. T. Brown, S. Guajardo, T. Devakul, S. S. Kondov, D. A. Huse, P. Schauß, and W. S. Bakr, "Quantum gas microscopy of an attractive Fermi-Hubbard system," Nature Phys. **276**, 238 (2017).

[S5] Z. Wu and E. Zaremba, "Dynamics of harmonically-confined systems: Some rigorous results," Ann. Phys. **342**, 214 (2014).

[S6] Quantum Electron Simulation Toolbox (QUEST) is an open source determinant quantum Monte Carlo toolbox. The package can be accessed via `http://quest.ucdavis.edu/index.html`.

[S7] G. J. A. Edge, R. Anderson, D. Jervis, D. C. McKay, R. Day, S. Trotzky, and J. H. Thywissen, "Imaging and addressing of individual fermionic atoms in an optical lattice," Phys. Rev. A **92**, 063406 (2015).

[S8] A. Tokuno and T. Giamarchi, "Spectroscopy for cold atom gases in periodically phase-modulated optical lattices," Phys. Rev. Lett. **106**, 205301 (2011).

[S9] H. D. Drew and P. Coleman, "Sum rule for the optical Hall angle," Phys. Rev. Lett. **78**, 1572 (1997).

[S10] L. J. LeBlanc, K. Jimenez-Garcia, R. A. Williams, M. C. Beeler, A. R. Perry, W. D. Phillips, and I. B. Spielman, "Observation of a superfluid Hall effect," Proc. Nat. Acad. Sci. **109**, 10811 (2012).

[S11] J. Y. Choi, S. Kang, S. W. Seo, W. J. Kwon, and Y. I. Shin, "Observation of a geometric Hall effect in a spinor bose-einstein condensate with a skyrmion spin texture," Phys. Rev. Lett. **111**, 245301 (2013).

[S12] D. T. Tran, A. Dauphin, A. G. Grushin, P. Zoller, and N. Goldman, "Probing topology by "heating": Quantized circular dichroism in ultracold atoms," Science Advances **3** (2017), 10.1126/sciadv.1701207.

[S13] L. Asteria, D. T. Tran, T. Ozawa, M. Tarnowski, B. S. Rem, N. Fläschner, K. Sengstock, N. Goldman, and C. Weitenberg, "Measuring quantized circular dichroism in ultracold topological matter," arXiv:1805.11077.

[S14] C. Hooley and J. Quintanilla, "Single-atom density of states of an optical lattice," Phys. Rev. Lett. **93**, 080404 (2004).

[S15] A. M. Rey, G. Pupillo, C. W. Clark, and C. J. Williams, "Ultracold atoms confined in an optical lattice plus parabolic potential: A closed-form approach," Phys. Rev. A **72**, 033616 (2005).

[S16] A. A. Abrikosov, *Fundamentals of the theory of metals* (North-Holland, Amsterdam, 1988).

[S17] G. Orso, L. P. Pitaevskii, and S. Stringari, "Umklapp collisions and center-of-mass oscillations of a trapped fermi gas," Phys. Rev. Lett. **93**, 020404 (2004).
